# Supplementary material for: Point-to-Point: Sparse Motion Guidance for Controllable Video Editing
Source: arXiv:2511.18277 source file (2025-11-23)
Supplement: Supplementary file 1 [file computation_cost_analysis.tex]

\section{Computation Cost Analysis}

\textbf{Memory Cost Analysis.} For anchor token selection, the memory cost includes 9GB for feature extraction~\cite{xiao2024video} and 9GB for optical flow estimation~\cite{teed2020raft}. During inference, anchor token alignment introduces no significant additional memory overhead beyond this baseline~\cite{guo2023animatediff, gu2024videoswap}, as anchor tokens operate in the latent space and similarity is computed over a reduced set of motion tokens.

\medskip
\noindent \textbf{Time Cost Analysis.} We analyze the time cost of anchor token selection and alignment. All time costs are calculated on an Nvidia A100 GPU to process a 16 frame video clip.
For anchor token selection, the time cost includes 30 seconds for feature extraction~\cite{xiao2024video}, 9 seconds for optical flow estimation~\cite{teed2020raft} and under 1 seconds for selecting anchor tokens. Anchor token alignment introduces an additional 10 seconds of computation time for calculating token distances and establishing correspondences. The remaining time cost remains similar to the base model~\cite{guo2023animatediff}, totaling 50 seconds.
