# Supplementary material for: Point-to-Point: Sparse Motion Guidance for Controllable Video Editing
Source: arXiv:2511.18277 source file (2025-11-23)
Supplement: Supplementary file 2 [file supp_trajectory.tex]

\begin{table}[!h]
\footnotesize
\setlength{\tabcolsep}{0.1em}
\definecolor{Gray}{gray}{0.9}

\begin{tabularx}{\linewidth}{m{3cm} | Y Y Y}
    \toprule
    & ViCLIP $\uparrow$ & Flow Sim. $\uparrow$ & Warp Err. $\downarrow$ \\
    \midrule\midrule
    \(\kappa=1\) & & & \\ %0.243 & 0.719 & 0.317 \\
    \(\kappa=\lfloor \frac{N}{2} \rfloor\) & & & \\ %0.248 & 0.733 & 0.316 \\
    \(\kappa=N\) & & & \\ %0.249 & 0.700 & 0.309 \\
    Ours & \textbf{0.257} & 0.711 & 0.336  \\
    \bottomrule
\end{tabularx}
\caption{Ablation study on anchor token alignment.}
\vspace{-0.5\baselineskip}
\label{tbl:supp_trajectory}
\end{table}
---------------------------------------- %
